# Supplementary material for: Prefill-Time Intervention for Mitigating Hallucination in Large Vision-Language Models
Source: arXiv:2604.25642 source file (2026-04-28)
Supplement: Supplementary file 1 [file appendix_pope_2model.tex]

\begin{table}[h]
    \centering
    \vspace{-5pt}
    \caption{More results of LLAVA-1.5 on POPE across distinct seeds, obtained under \textbf{Sampling Decoding (top-p=1.0)}.}
    \vspace{-10pt}
    \resizebox{1\linewidth}{!}{%
    \begin{tabular}{cc cccc cccc}
        \whline
        % Method  & LLAVA.  &  {Qwen.}  &  {DeepSeek.} \\
        \multirow{2}{*}{Seed}            
        & \multirow{2}{*}{Method}            
        & \multicolumn{2}{c}{Random}
        & \multicolumn{2}{c}{Popular}
        & \multicolumn{2}{c}{Adversarial}
        & \multicolumn{2}{c}{Avg} \\
        
        \cmidrule(r){3-4} \cmidrule(r){5-6} \cmidrule(r){7-8} \cmidrule(r){9-10} 

        % & & Ran. & Pop. & Adv. & Avg
        %  & Ran. & Pop. & Adv. & Avg \\
         ~ & & $\text{Acc} \uparrow$  & $\text{F1} \uparrow$  &  $\text{Acc} \uparrow$  & $\text{F1} \uparrow$  &  $\text{Acc} \uparrow$  & $\text{F1} \uparrow$   &  $\text{Acc} \uparrow$  & $\text{F1} \uparrow$  \\
          
        \hline
        % --- 第一组 ---
        % 注意：\rowcolor 必须放在 \multirow 之前
        % \rowcolor{mygray}
        % \multirow{3}{*}{2000} 
        \multirow{3}{*}{\makecell{1994 \\ (default)}}
        & Vanilla &  \cellcolor{mygray}$83.74$ &  \cellcolor{mygray}$84.54$ &  \cellcolor{mygray}$80.50$ &  \cellcolor{mygray}$81.49$ &  \cellcolor{mygray}$75.40 $ & \cellcolor{mygray}$ 77.67$ & \cellcolor{mygray}$79.88$ & \cellcolor{mygray}$81.23$ \\
        &  VTI  & $83.40$ & $84.14$ & $81.50$ & $82.33$ & $76.33$ &$ 78.47$ & $80.41$ & $81.64$ \\
        &  PTI (ours) & \cellcolor{myblue}$\bold{85.43}$ & \cellcolor{myblue}$\bold{85.72}$ & \cellcolor{myblue}$\bold{83.80}$ & \cellcolor{myblue}$\bold{84.09}$ & \cellcolor{myblue}$\bold{77.40}$   & \cellcolor{myblue}$\bold{78.75}$ & \cellcolor{myblue}$\bold{82.21}$ & \cellcolor{myblue}$\bold{82.85}$\\

        \hline
        % --- 第二组 ---
        % \rowcolor{mygray}
        \multirow{3}{*}{2026} 
        & Vanilla &  \cellcolor{mygray}$82.99$ & \cellcolor{mygray}$83.78$ & \cellcolor{mygray}$81.60$ & \cellcolor{mygray}$82.53$ & \cellcolor{mygray}$76.63$ & \cellcolor{mygray}$78.75$ & \cellcolor{mygray}$80.41$ & $\cellcolor{mygray}81.69$ \\
        &  VTI  & $83.54$ & $83.97$ & $81.37$ & $81.88$ & $76.23$ & $77.93$ & $80.38$ & $81.26$ \\
        &  PTI (ours) &  \cellcolor{myblue}$\bold{84.62}$ & \cellcolor{myblue}$\bold{84.94}$ & \cellcolor{myblue}$\bold{83.36}$ & \cellcolor{myblue}$\bold{83.68}$ & \cellcolor{myblue}$\bold{77.00}$ & \cellcolor{myblue}$\bold{78.50}$ & \cellcolor{myblue}$\bold{81.66}$ & \cellcolor{myblue}$\bold{82.37}$ \\ 
         
        \hline
        % --- 第三组 ---
        % \rowcolor{mygray}
        \multirow{3}{*}{42} & Vanilla & \cellcolor{mygray}$83.57$ & \cellcolor{mygray}$84.20$ & \cellcolor{mygray}$80.37$ & \cellcolor{mygray}$81.46$ & \cellcolor{mygray}$75.30$ & \cellcolor{mygray}$77.58$ & \cellcolor{mygray}$79.75$ & \cellcolor{mygray}$81.08$ \\
        &  VTI  & $84.33$ & $84.72$ & $80.47$ & $81.11$ & $75.99$ & $77.79$ & $80.26$ & $81.21$ \\
        &  PTI (ours) & \cellcolor{myblue}$\bold{85.36}$ & \cellcolor{myblue}$\bold{85.57}$ & \cellcolor{myblue}$\bold{83.80}$ & \cellcolor{myblue}$\bold{83.34}$ & \cellcolor{myblue}$\bold{76.73}$ & \cellcolor{myblue}$\bold{78.42}$ & \cellcolor{myblue}$\bold{81.96}$ & \cellcolor{myblue}$\bold{82.44}$ \\

        \whline
    \end{tabular}}
    % \vspace{-12pt}
    \vspace{-10pt}
    \label{tab:reb_pope}
\end{table}
