# Supplementary material for: Prefill-Time Intervention for Mitigating Hallucination in Large Vision-Language Models
Source: arXiv:2604.25642 source file (2026-04-28)
Supplement: Supplementary file 2 [file appendix.tex]

% CVPR 2026 Paper Template; see https://github.com/cvpr-org/author-kit

\documentclass[10pt,twocolumn,letterpaper]{article}

%%%%%%%%% PAPER TYPE  - PLEASE UPDATE FOR FINAL VERSION
% \usepackage{cvpr}              % To produce the CAMERA-READY version
\usepackage[review]{cvpr}      % To produce the REVIEW version
\usepackage{amsmath,amssymb,amsfonts}
\usepackage{algorithmic}
\usepackage{graphicx}
\usepackage{textcomp}
\usepackage{xcolor}
\usepackage[table]{xcolor}
\usepackage{color,colortbl}
\usepackage{wrapfig}
\usepackage{array}
\usepackage{bbding}
\usepackage{arydshln}
\usepackage{amsmath}
\usepackage{amssymb}
\usepackage{graphicx}
\usepackage{booktabs}
\usepackage{CJKutf8}
\usepackage{multirow}
\usepackage{enumitem} % 在导言区添加
\usepackage{makecell}
\usepackage{bbm}
\usepackage{arydshln}
\usepackage[normalem]{ulem}

\newcommand{\tocite}[1]{{\textcolor{red}{TOCITE}}}

\newcolumntype{I}{!{\vrule width 1.2pt}}
\newlength\savedwidth

\newlength\savewidth

\newcommand{\s}[1]{}
\definecolor{darkergreen}{RGB}{21, 152, 56}
\newcommand\greenp[1]{\textcolor{darkergreen}{}}
\usepackage[linesnumbered,ruled,vlined]{algorithm2e}
% \newcommand{\todo}[1]{{\textcolor{red}{#1}}}

% Import additional packages in the preamble file, before hyperref
\input{preamble}

% It is strongly recommended to use hyperref, especially for the review version.
% hyperref with option pagebackref eases the reviewers' job.
% Please disable hyperref *only* if you encounter grave issues, 
% e.g. with the file validation for the camera-ready version.
%
% If you comment hyperref and then uncomment it, you should delete *.aux before re-running LaTeX.
% (Or just hit 'q' on the first LaTeX run, let it finish, and you should be clear).
\definecolor{cvprblue}{rgb}{0.21,0.49,0.74}
\definecolor{newcolor}{rgb}{.8,.349,.1}
\definecolor{mypink}{rgb}{.99,.91,.95}
% \definecolor{mygreen}{RGB}{107,147,147}
\definecolor{mygreen}{RGB}{26,104,64}
\definecolor{lgreen}{HTML}{00b8a9}
\definecolor{mygray}{HTML}{eeeeee}
\definecolor{myred}{HTML}{fae4df}
\definecolor{mydarkred}{HTML}{ed3333}
\definecolor{mydarkgray}{HTML}{808080}
\definecolor{myblue}{HTML}{E0F0FA}
\definecolor{mypink}{rgb}{0,0,0}

\usepackage[pagebackref,
            breaklinks,
            colorlinks,
            allcolors=cvprblue,
            linkcolor=cvprblue,  
            anchorcolor=cvprblue,
            citecolor=cvprblue,
            ]{hyperref}

%%%%%%%%% PAPER ID  - PLEASE UPDATE
 % *** Enter the Paper ID here

%%%%%%%%% TITLE - PLEASE UPDATE
\title{PTI: Prefill-Time Intervention for Mitigating Hallucination in Large Vision-Language Models}

%%%%%%%%% AUTHORS - PLEASE UPDATE
% \author{First Author\\
% Institution1\\
% Institution1 address\\
% {\tt\small firstauthor@i1.org}
% % For a paper whose authors are all at the same institution,
% % omit the following lines up until the closing ``}''.
% % Additional authors and addresses can be added with ``\and'',
% % just like the second author.
% % To save space, use either the email address or home page, not both
% \and
% Second Author\\
% Institution2\\
% First line of institution2 address\\
% {\tt\small secondauthor@i2.org}
% }

\begin{document}
\maketitlesupplementary
\input{sec/X_suppl}

{
    \small
    \bibliographystyle{ieeenat_fullname}
    \bibliography{main}
}

% WARNING: do not forget to delete the supplementary pages from your submission 
% \input{sec/X_suppl}

\end{document}
