# Supplementary material for: Prefill-Time Intervention for Mitigating Hallucination in Large Vision-Language Models
Source: arXiv:2604.25642 source file (2026-04-28)
Supplement: Supplementary file 3 [file appendix_comp.tex]

\begin{table}[h]
    \centering
    \vspace{-5pt}
    % 注意：你的标题写的是 Latency，但表格内容是 Accuracy/CHAIR 指标，建议修改标题
    \caption{Comparison of performance with more recent works under \textbf{Greedy Decoding} for fairness.
    % on POPE, CHAIR, and MME.
        $^{\dagger}$: the results from their papers.
    } 
    \vspace{-10pt}
    \resizebox{1\linewidth}{!}{%
    % 修改 1: 根据实际内容，将列数改为 6 列 (lccccc)
    \begin{tabular}{lccccc} 
        \whline % 修改 2: 使用标准的 \toprule 替换 \whline
        \multirow{2}{*}{Method}            
        & \multicolumn{2}{c}{POPE} 
        & \multicolumn{2}{c}{CHAIR} 
        & MME \\ % 修改 3: MME 下方只有一个 Score，所以这里设为 1 列
        
        \cmidrule(r){2-3} \cmidrule(r){4-5}  \cmidrule(r){6-6}  

         & $\text{Acc } \uparrow$ & $\text{F1 } \uparrow $ 
         & $\text{CHAIR}_S \downarrow$ & $\text{CHAIR}_I \downarrow$ 
         & $\text{Score }  \uparrow$  \\
         
        \hline % 使用 \midrule 替换 \hline
        
        % 修改 4: 补全所有行的 & 占位符，确保列对齐
\rowcolor{mygray}        
Vanilla (Greedy) & $84.87$ & $85.59$ & $47.4$ & $13.7$ & $611.6$ \\

VASparse (CVPR2025) \footnotemark[4] $^{\dagger}$ &$70.84$ & $60.08$ & $18.51$ & $5.82$ & $594$ \\
        
MemVR (ICML2025) \footnotemark[5] $^{\dagger}$  &$86.93$ & $85.88$ & $46.6$ & $13$ & $648.3$\\

SENTINEL (ICCV2025) \footnotemark[6] $^{\dagger}$  & N/A & N/A & N/A & N/A & N/A \\

\rowcolor{myblue}
\textbf{PTI (ours)}  & $\bold{87.10}$  & $\bold{86.88}$  & $\bold{15.4}$ & $\bold{5.4}$ & $\bold{651.6}$\\ 

        \whline % 使用 \bottomrule 替换 \whline
    \end{tabular}}
    \vspace{-10pt}
    \label{tab:appendix_performance} % 修改 label 以匹配内容
\end{table}
