# Supplementary material for: Prefill-Time Intervention for Mitigating Hallucination in Large Vision-Language Models
Source: arXiv:2604.25642 source file (2026-04-28)
Supplement: Supplementary file 4 [file appendix_latency.tex]

\begin{table}[h]
    \centering
    \caption{Measure of Latency (ms/token) and Throughput (token/s).}
    \vspace{-8pt}
    \resizebox{1\linewidth}{!}{%
    % \begin{tabular}{lccccccc}
    \begin{tabular}{lccccc}
        \whline
        % Method  & LLAVA.  &  {Qwen.}  &  {DeepSeek.} \\
        \multirow{2}{*}{Method}           
        & \multicolumn{2}{c}{LLAVA-1.5} 
        % & \multicolumn{2}{c}{Qwen-VL-Chat} 
        & \multicolumn{2}{c}{DeepSeek-VL-Chat} \\
        
        % \cmidrule(r){2-3} \cmidrule(r){4-5}  \cmidrule(r){6-7}  
        \cmidrule(r){2-3} \cmidrule(r){4-5}  

         & $\text{Latency   } \downarrow$ & $\text{Throughput } \uparrow $ 
         % & $\text{Latency } \downarrow$ & $\text{Throughput } \uparrow $ 
         & $\text{Latency }  \downarrow$ & $\text{Throughput } \uparrow $  \\

        % \cline{2-5}
        % \cmidrule(r){2-3} \cmidrule(r){4-5}  

               % &  Latency & Throughput & Latency & Throughput  \\
\hline
\rowcolor{mygray}
Vanilla (Sampling 1.0) 
&\tabincell{c}{$19.52$ ($\times1.00)$}   
&\tabincell{c}{$51.22$ ($\times 1.00$)}
% & \tabincell{c}{$20.55$  ($\times1.00$)} 
% &\tabincell{c}{$48.66$ ($\times1.00$)}
& \tabincell{c}{$18.29$  ($\times1.00$)}
& \tabincell{c}{$54.67$  ($\times1.00$)}
\\

VCD (CVPR2024) % \cite{leng2024mitigating} 
&\tabincell{c}{$38.92$ \color{mydarkgray}($\times1.99$)}  
& \tabincell{c}{$25.69$ \color{mydarkgray}($\times0.50$)}
% &  \tabincell{c}{$41.08$ \color{mydarkgray}($\times1.99$)}
% &\tabincell{c}{$24.34$ \color{mydarkgray}($\times0.50$)}
& \tabincell{c}{$36.38$ \color{mydarkgray}($\times1.98$)}
&\tabincell{c}{$27.49$ \color{mydarkgray}($\times0.50$)}
\\

% PAI \cite{liu2024paying} 
% & \tabincell{c}{$37.62$ \color{mydarkgray}($\times1.93$)}  
% &\tabincell{c}{$26.58$ \color{mydarkgray}($\times0.52$)}
% % & \tabincell{c}{$42.07$ \color{mydarkgray}($\times2.04$)} 
% % & \tabincell{c}{$23.77$ \color{mydarkgray}($\times0.48$)}
% & \tabincell{c}{$35.16$ \color{mydarkgray}($\times1.92$)} 
% &\tabincell{c}{$28.44$ \color{mydarkgray}($\times0.52$)} \\

VISTA (ICML2025) % \cite{li2025hidden} 
&\tabincell{c}{$26.20$ \color{mydarkgray}($\times1.34$)}   
&\tabincell{c}{$38.17$ \color{mydarkgray}($\times0.74$)}
% &\tabincell{c}{$33.81$ \color{mydarkgray}($\times1.64$)} 
% &\tabincell{c}{$29.57$ \color{mydarkgray}($\times0.60$)}
& \tabincell{c}{$26.79$ \color{mydarkgray}($\times1.46$)}
&\tabincell{c}{$37.33$ \color{mydarkgray}($\times0.68$)} \\

VTI (ICLR2025) % \cite{liu2024reducing} 
& \tabincell{c}{$20.84$ \color{mydarkgray}($\times1.07$)}
&\tabincell{c}{$47.97$ \color{mydarkgray}($\times0.93$)}
% & \tabincell{c}{$21.86$ \color{mydarkgray}($\times1.06$)} 
% &\tabincell{c}{$45.75$ \color{mydarkgray}($\times0.94$)}
& \tabincell{c}{$19.81$ \color{mydarkgray}($\times1.08$)}  
&\tabincell{c}{$50.47$ \color{mydarkgray}($\times0.92$)} \\

\rowcolor{myblue}
\textbf{PTI (ours) }
& \tabincell{c}{$\bold{19.58}$ \color{mygreen}($\times \bold{1.00}$)} 
& \tabincell{c}{$\bold{51.06}$ \color{mygreen}($\times \bold{0.99}$)} 
% & \tabincell{c}{$\bold{20.88}$ \color{mygreen}($\times \bold{1.01}$)} 
% & \tabincell{c}{$\bold{47.90}$ \color{mygreen}($\times \bold{0.98}$)}
& \tabincell{c}{$\bold{18.56}$ \color{mygreen}($\times \bold{1.02}$)}  
& \tabincell{c}{$\bold{53.89 }$ \color{mygreen}($\times \bold{0.99}$)}  \\

        \whline
    \end{tabular}}
	\vspace{-10pt}
    \label{tab:reb_latency}
\end{table}
